# Supplementary material for: Regularized Mask Tuning: Uncovering Hidden Knowledge in Pre-trained Vision-Language Models
Source: arXiv:2307.15049 source file (2023-08-06)
Supplement: Supplementary file 1 [file ppl_appendix.tex]

\appendix
\clearpage
\onecolumn

\section{Limitations and Broader Impact}
\noindent\textbf{Broader Impact.} As for positive impact,  we design a novel parameter prompt strategy to select a subset of network parameters in pre-trained model for few-shot visual recognition tasks. 
The learned parameter prompts can further boost the transfer capacity of the existing prompt-based and adapter-based methods.

\noindent\textbf{Limitations.} As for limitations, our method, as a general method, has not been verified on open-world detection and segmentation tasks due to limited computational resources. We leave this exploration in the future.

% \section{Additional Implementation Details}
% % The learning rate is set to be 9e-5 for ImageNet
% To train parameter prompts when using ViT as visual backbone, the weight decay of Adam optimizer is set to be 5e-4 for 16-shot ImageNet. The maximum training epoch is 10.

\section{Preliminaries of CLIP-related Tuning Methods}

To improve the transferability in the various downstream tasks, some parameter-efficient studies based on these V\&L models, \textit{e.g.}, adapter~\cite{gao2021clip,zhang2022tip} or prompt~\cite{zhou2022learning,zang2022unified}, are proposed. Specifically, Zhou \etal~\cite{zhou2022learning} change the hand-craft text prompt to a task-specific learnable \textit{text prompt}, which can be formulated as ``$[\boldsymbol{T}_1] [\boldsymbol{T}_2] \cdots [\boldsymbol{T}_l][class]$''. Here, the $l$ refers to the length of the learnable text prompt. The text encoder extracts text features $\boldsymbol{w}\prime_i$ from the learned text prompt to match the image features, which is the same as~\cref{eq.possibility}. The learnable text prompt is optimized with cross-entropy classification loss. 
% Zang \etal \cite{zang2022unified} introduce a unified prompt into both the text and image branches. The unified prompt is also a set of learnable parameters $\boldsymbol{U}\in \mathcal{R}^{d*l}$, where the $d$, $l$ denote the dimension and length of the prompt, respectively. Then the unified prompt is refined by a transformer layer and split into two parts to complete the image and text input, which can be formulated as follows:
% \begin{gather}
%     \label{eq.unified_prompt}
%     \boldsymbol{U}' = transformer(\boldsymbol{U}),  \\
%     \{\boldsymbol{U}_t, \boldsymbol{U}_v\} = \boldsymbol{U}',
% \end{gather}
% where the $\boldsymbol{U}_t, \boldsymbol{U}_v$ denote text prompt and visual prompt, respectively. Then the prompts are combined with text or image to be used as input for CLIP.
For the adapter-based method, Zhang \etal~\cite{zhang2022tip} build an adapter following the image encoder of CLIP. Given $S$-shot training data, the weights of adapter $\boldsymbol{A}$ are initialized with the few-shot image features $\boldsymbol{F}_I\in\mathcal{R}^{m\times d}$ encoded by the image encoder $\boldsymbol{G}_I$. The ground truth labels of images are converted into a one-hot vector $\boldsymbol{L}_I\in\mathcal{R}^{m\times k}$. The possibility of assigning image $\boldsymbol{x}_j$ to class $\boldsymbol{y}_i$ can be formulated as:
\begin{gather}
    \label{eq.tip}
    p_t(\boldsymbol{y}=i\mid \boldsymbol{x}_j)=\alpha \boldsymbol{A}(\boldsymbol{f}_j)\boldsymbol{L}_I^i+p(\boldsymbol{y}=i \mid \boldsymbol{x}_j), \\
    \boldsymbol{A}(\boldsymbol{f}_j) = exp(-\beta(1-\boldsymbol{f}_j\boldsymbol{F}^\mathrm{T}_I)),
    % \boldsymbol{f}_j\boldsymbol{F}^\mathrm{T}_{I_i})
\end{gather}
where the $\alpha$ and $\beta$ are hyper-parameters, $\boldsymbol{L}_I^i\in\mathcal{R}^{m\times 1}$ denotes $i$-th column of $\boldsymbol{L}_I$, which corresponds to class $i$. The TIP-Adapter achieves better performance when fine-tuning the adapter $\boldsymbol{A}$ with $S$-shot training.

\subsection{Comparison to State-of-the-Art Methods}

\begin{figure*}[t]
\centering 
\subfloat[\textbf{Average over 11 datasets}]{
     \centering
     \includegraphics[width=0.30\linewidth,height=0.22\linewidth]{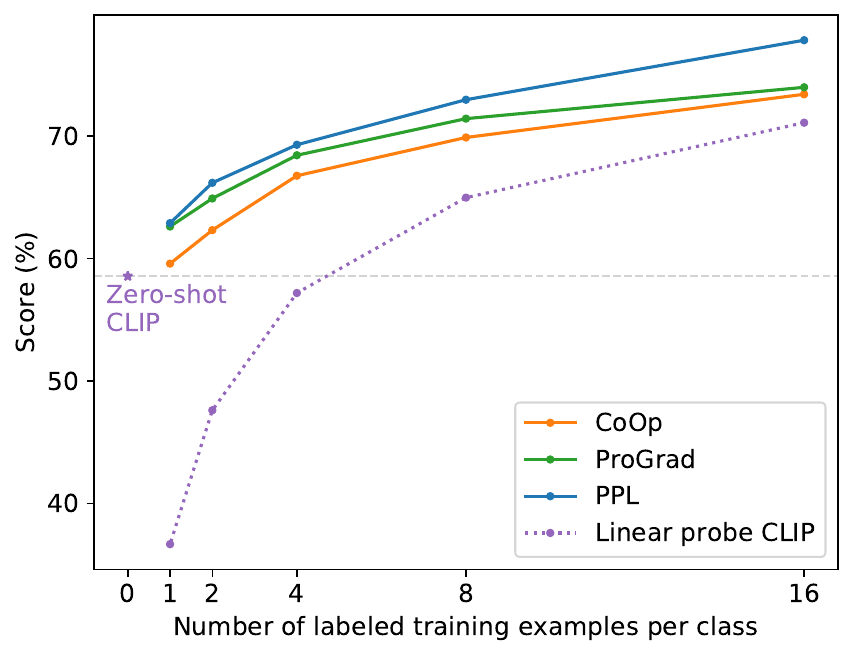}
     \label{fig:rn50_Average}
 }
 \hfill
\subfloat[FGVCAircraft]{
     \centering
     \includegraphics[width=0.30\linewidth,height=0.22\linewidth]{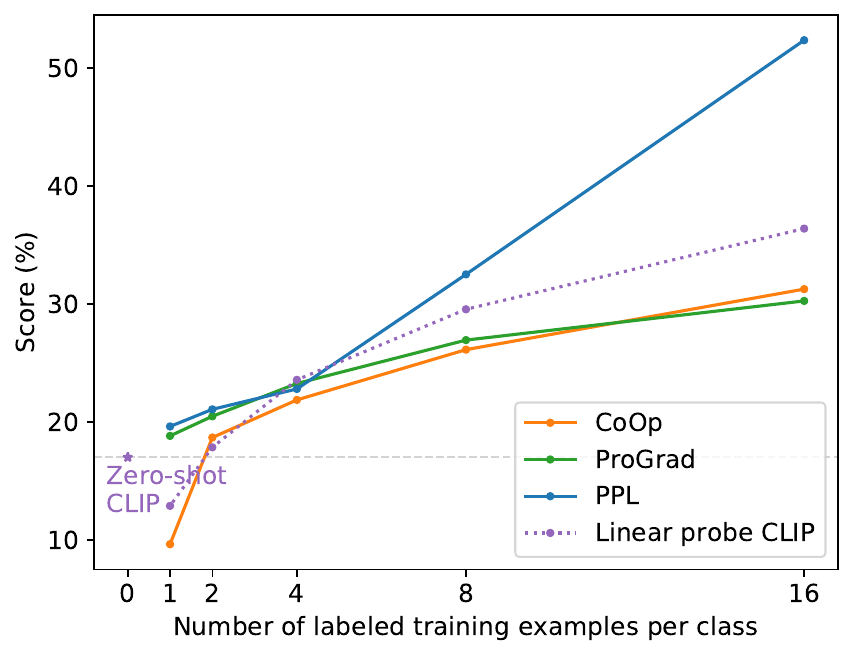}
     \label{fig:rn50_FGVCAircraft}
}
\hfill
\subfloat[ImageNet]{
     \centering
     \includegraphics[width=0.30\linewidth,height=0.22\linewidth]{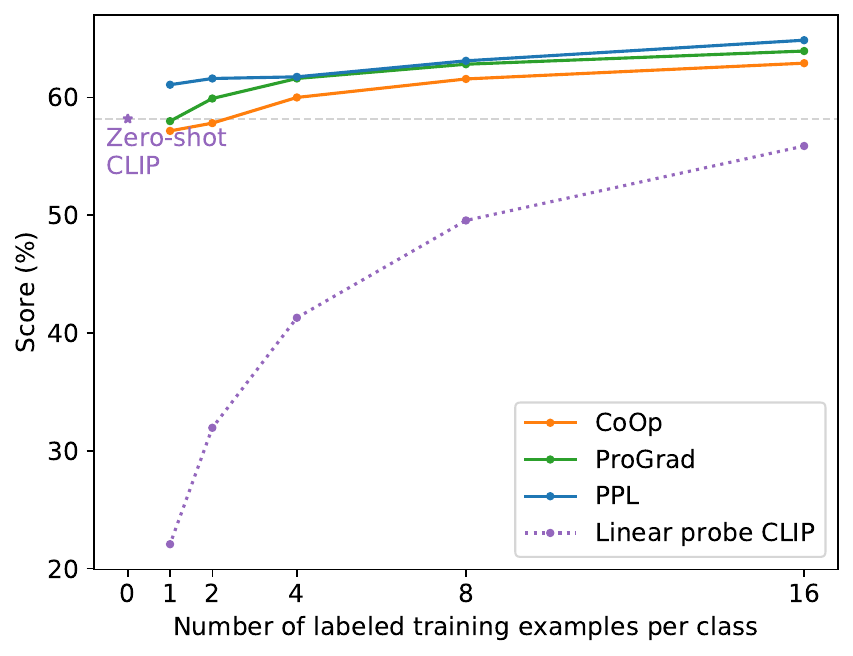}
     \label{fig:rn50_ImageNet}
}
\vspace{-10pt}
\subfloat[StanfordCars]{
     \centering
     \includegraphics[width=0.30\linewidth,height=0.22\linewidth]{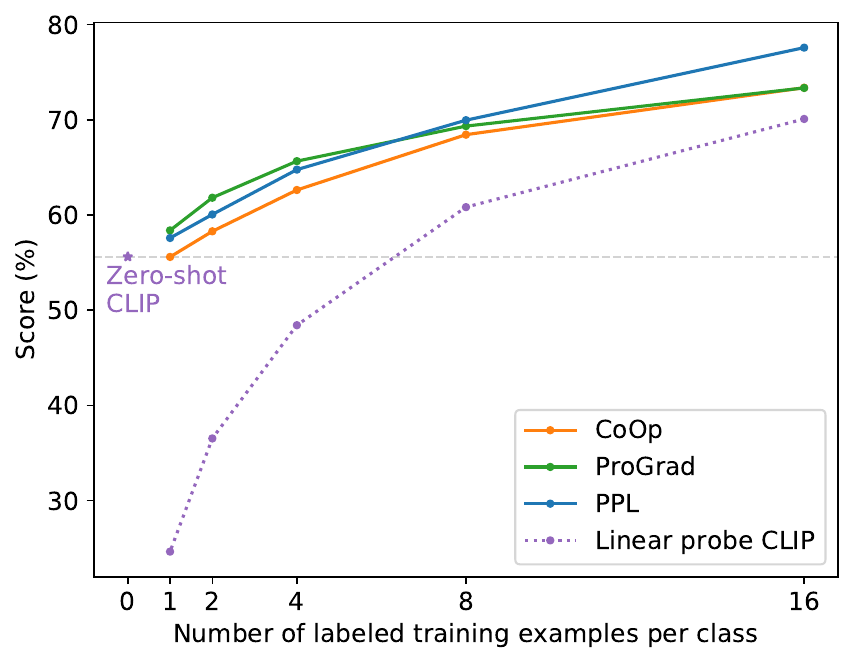}
     \label{fig:rn50_StanfordCars}
}
\hfill
\subfloat[Caltech101]{
     \centering
     \includegraphics[width=0.30\linewidth,height=0.22\linewidth]{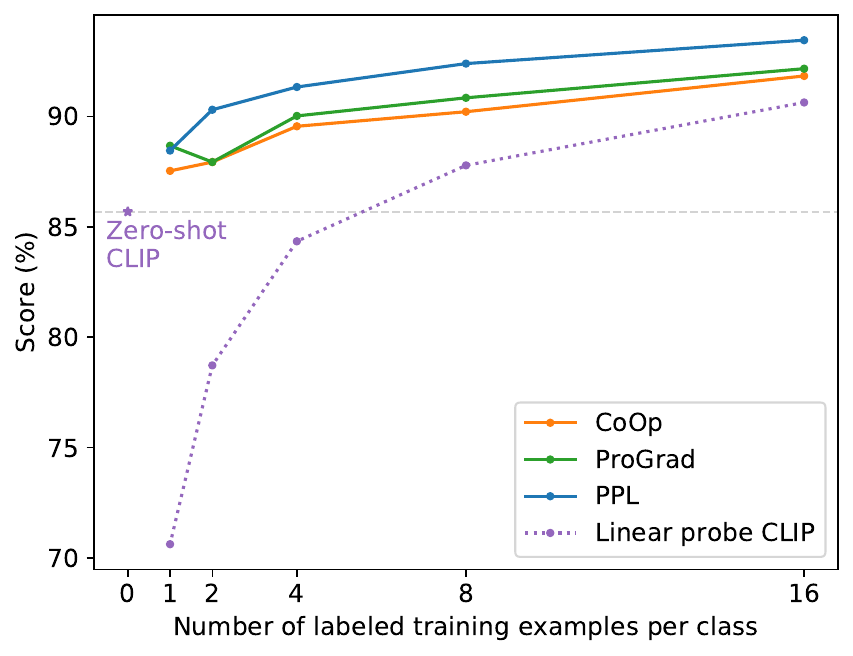}
     \label{fig:rn50_Caltech101}
}
\hfill
\subfloat[UCF101]{
     \centering
     \includegraphics[width=0.30\linewidth,height=0.22\linewidth]{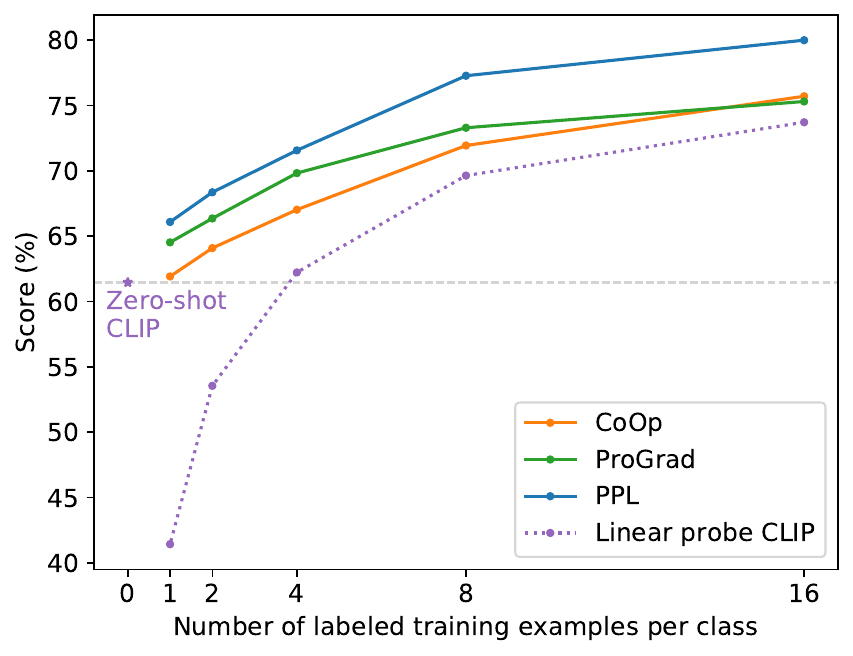}
     \label{fig:rn50_UCF101}
}
\vspace{-10pt}
\subfloat[EuroSAT]{
     \centering
     \includegraphics[width=0.30\linewidth,height=0.22\linewidth]{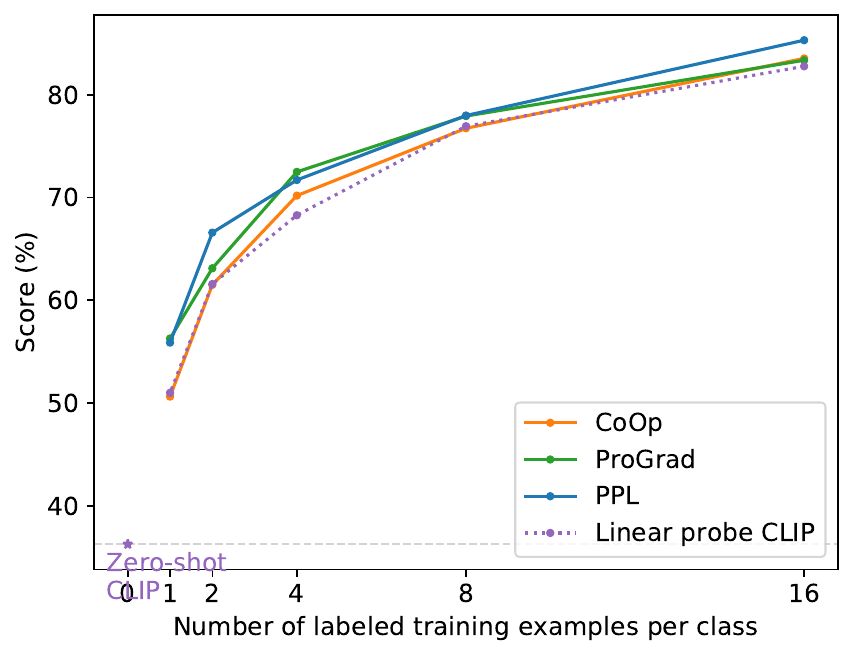}
     \label{fig:rn50_EuroSAT}
}
\hfill
\subfloat[Flowers102]{
     \centering
     \includegraphics[width=0.30\linewidth,height=0.22\linewidth]{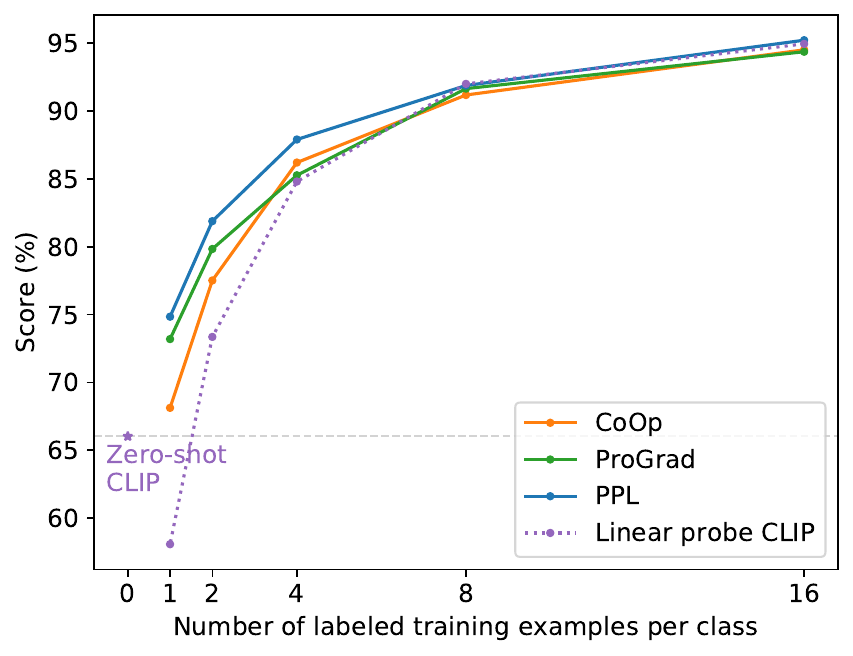}
     \label{fig:rn50_Flowers102}
}
\hfill
\subfloat[Food101]{
     \centering
     \includegraphics[width=0.30\linewidth,height=0.22\linewidth]{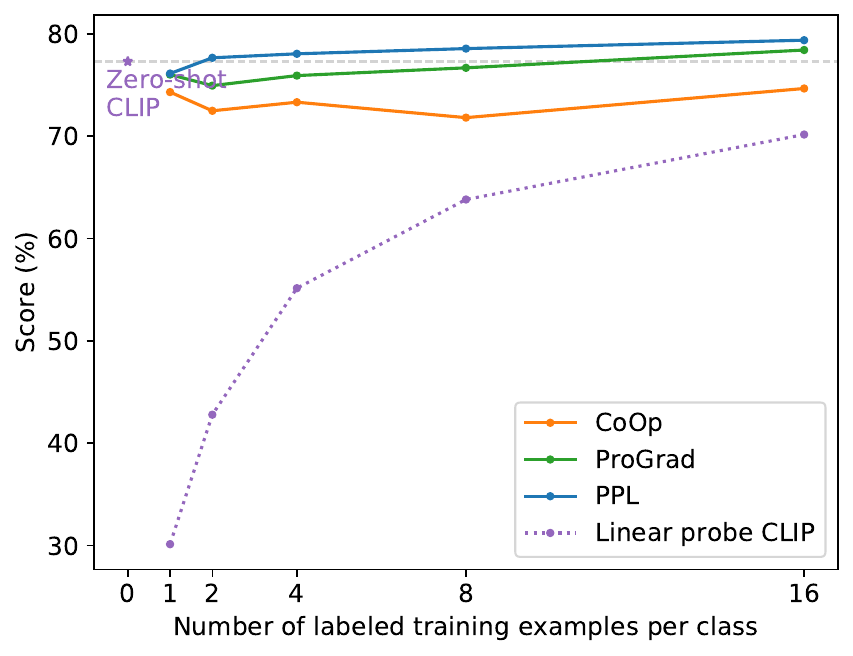}
     \label{fig:rn50_Food101}
}
\vspace{-10pt}
\subfloat[SUN397]{
     \centering
     \includegraphics[width=0.30\linewidth,height=0.22\linewidth]{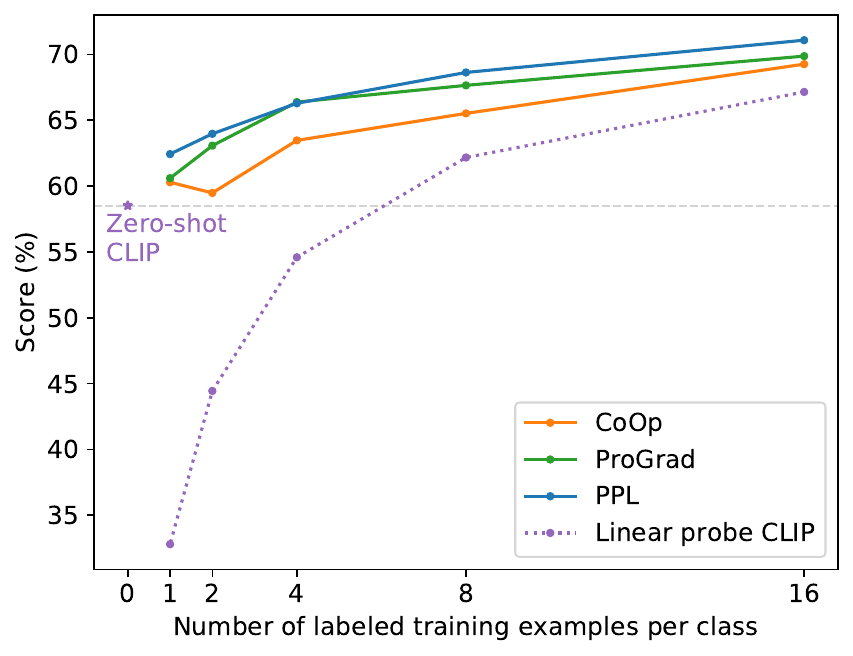}
     \label{fig:rn50_SUN397}
}
\hfill
\subfloat[OxfordPets]{
     \centering
     \includegraphics[width=0.30\linewidth,height=0.22\linewidth]{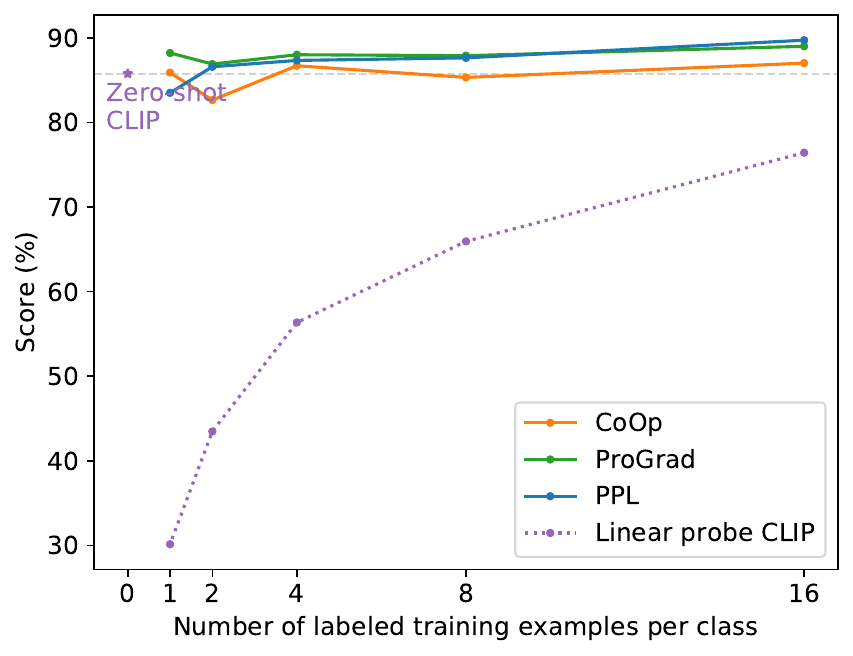}
     \label{fig:rn50_OxfordPets}
}
\hfill
\subfloat[DTD]{
     \centering
     \includegraphics[width=0.30\linewidth,height=0.22\linewidth]{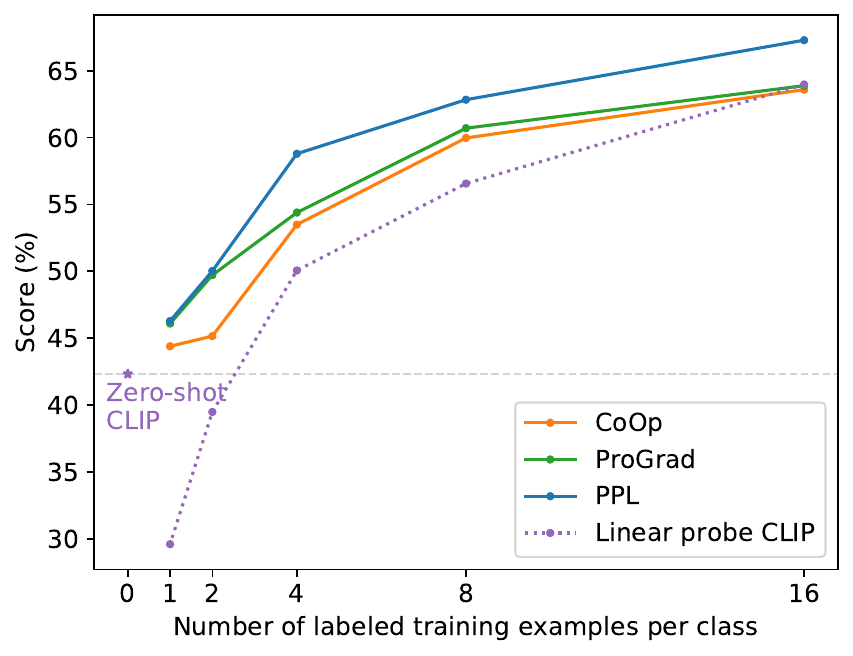}
     \label{fig:rn50_DTD}
}
\vspace{5pt}
\caption{ \textbf{Accuracy (\%) of few-shot learning, \ie, 16/8/4/2/1-shot, on the 11 datasets.} We report the average accuracy over three runs. For AMT, R-AMT, and TIP-Adapter, we demonstrate the \textit{error bar} in all figures.}
\label{fig:main_results_vit} 
\vspace{-.1in}
\end{figure*}

\iffalse
\begin{figure*}[t]
\centering 
\begin{subfigure}[b]{0.33\linewidth}
     \centering
     \includegraphics[width=\linewidth]{fig/Average.pdf}
     \caption{Average}
     \label{fig:rn50_Average}
\end{subfigure}
\begin{subfigure}[b]{0.33\linewidth}
     \centering
     \includegraphics[width=\linewidth]{fig/FGVCAircraft.pdf}
     \caption{FGVCAircraft}
     \label{fig:rn50_FGVCAircraft}
\end{subfigure}
\begin{subfigure}[b]{0.33\linewidth}
     \centering
     \includegraphics[width=\linewidth]{fig/ImageNet.pdf}
     \caption{ImageNet}
     \label{fig:rn50_ImageNet}
\end{subfigure}

\begin{subfigure}[b]{0.33\linewidth}
     \centering
     \includegraphics[width=\linewidth]{fig/StanfordCars.pdf}
     \caption{StanfordCars}
     \label{fig:rn50_StanfordCars}
\end{subfigure}
\begin{subfigure}[b]{0.33\linewidth}
     \centering
     \includegraphics[width=\linewidth]{fig/Caltech101.pdf}
     \caption{Caltech101}
     \label{fig:rn50_Caltech101}
\end{subfigure}
\begin{subfigure}[b]{0.33\linewidth}
     \centering
     \includegraphics[width=\linewidth]{fig/UCF101.pdf}
     \caption{UCF101}
     \label{fig:rn50_UCF101}
\end{subfigure}

\begin{subfigure}[b]{0.33\linewidth}
     \centering
     \includegraphics[width=\linewidth]{fig/EuroSAT.pdf}
     \caption{EuroSAT}
     \label{fig:rn50_EuroSAT}
\end{subfigure}
\begin{subfigure}[b]{0.33\linewidth}
     \centering
     \includegraphics[width=\linewidth]{fig/Flowers102.pdf}
     \caption{Flowers102}
     \label{fig:rn50_Flowers102}
\end{subfigure}
\begin{subfigure}[b]{0.33\linewidth}
     \centering
     \includegraphics[width=\linewidth]{fig/Food101.pdf}
     \caption{Food101}
     \label{fig:rn50_Food101}
\end{subfigure}

\begin{subfigure}[b]{0.33\linewidth}
     \centering
     \includegraphics[width=\linewidth]{fig/SUN397.pdf}
     \caption{SUN397}
     \label{fig:rn50_SUN397}
\end{subfigure}
\begin{subfigure}[b]{0.33\linewidth}
     \centering
     \includegraphics[width=\linewidth]{fig/OxfordPets.pdf}
     \caption{OxfordPets}
     \label{fig:rn50_OxfordPets}
\end{subfigure}
\begin{subfigure}[b]{0.33\linewidth}
     \centering
     \includegraphics[width=\linewidth]{fig/DTD.pdf}
     \caption{DTD}
     \label{fig:rn50_DTD}
\end{subfigure}
\caption{Accuracy of few-shot learning on the 11 datasets using ResNet-50 as the architecture of image encoder.}
\label{fig:rn50_main_results}
\vspace{-.1in}
\end{figure*}

\noindent
\textbf{Accuracy on 11 Datasets.} We compare PPL with two baseline methods and two state-of-the-art prompt-based methods on the aforementioned 11 datasets, which are demonstrated in \cref{fig:main_results}. 
% It is mentioned that although the VPT and UPT adopt the visual/unified prompt, they are only for transformer architecture to design methods and are not universal. Thus, we do not include the VPT and UPT in this setting of 11 Datasets.
The baseline methods include Zero-shot CLIP and Linear probe CLIP: 1) the former directly transfers to the downstream task without training; 2) the latter trains a linear classifier for downstream tasks based on the pretrained CLIP. The prompt-based methods are CoOP~\cite{zhou2022learning} and ProGrad~\cite{zhu2022prompt}. Both of them tend to learn better text prompts for adaptation to downstream tasks. 
According to~\cref{fig:Average}, the PPL outperforms these methods on average over 11 datasets, which approves the ability of PPL to transfer CLIP to the downstream tasks with few-shot data. Concretely, the PPL improves the second-best method ProGrad by 3.85\% on the 16-shot setting, while 33.50\% of parameters in the image encoder are left out on average.
Moreover, the PPL achieves the best accuracy in most of the datasets on the 16/8/4/2-shot setting. From \cref{fig:FGVCAircraft}, we find the improvement in terms of accuracy is more significant as the training few-shot data increase for the FGVCAircraft dataset.
However, given the 1-shot data for training, there is performance degradation of PPL on some datasets, \eg Food101. This shows the reliability of the parameter prompt depends on the number of training data. A small quantity of training data for fine-grained classification tasks may lead to overfitting.
% to select preferred knowledge within the pretrained model for downstream tasks.

\noindent\textbf{Comparison with Zero-shot CLIP.}
In \cref{fig:compare_zs_rn50}, we demonstrate the absolute improvement of PPL compared with Zero-shot CLIP and the sparsity of parameter prompts on the 16-shot setting. The PPL boosts the performance of Zero-shot CLIP on all datasets.  Significant improvements were achieved on EuroSAT and FGVCAircraft dataset, which reach 49.03\% and 35.35\%, respectively. For FGVCAircraft, the sparsity of parameter prompts reaches 73.47\% (\ie, the 73.47 percentage of zeros in binary masks). It proves that the pre-trained weights contain some unnecessary information for the downstream task, which may harm the transfer ability of the pre-trained model.

\begin{figure}[t]
    \centering
    \includegraphics[scale=0.43]{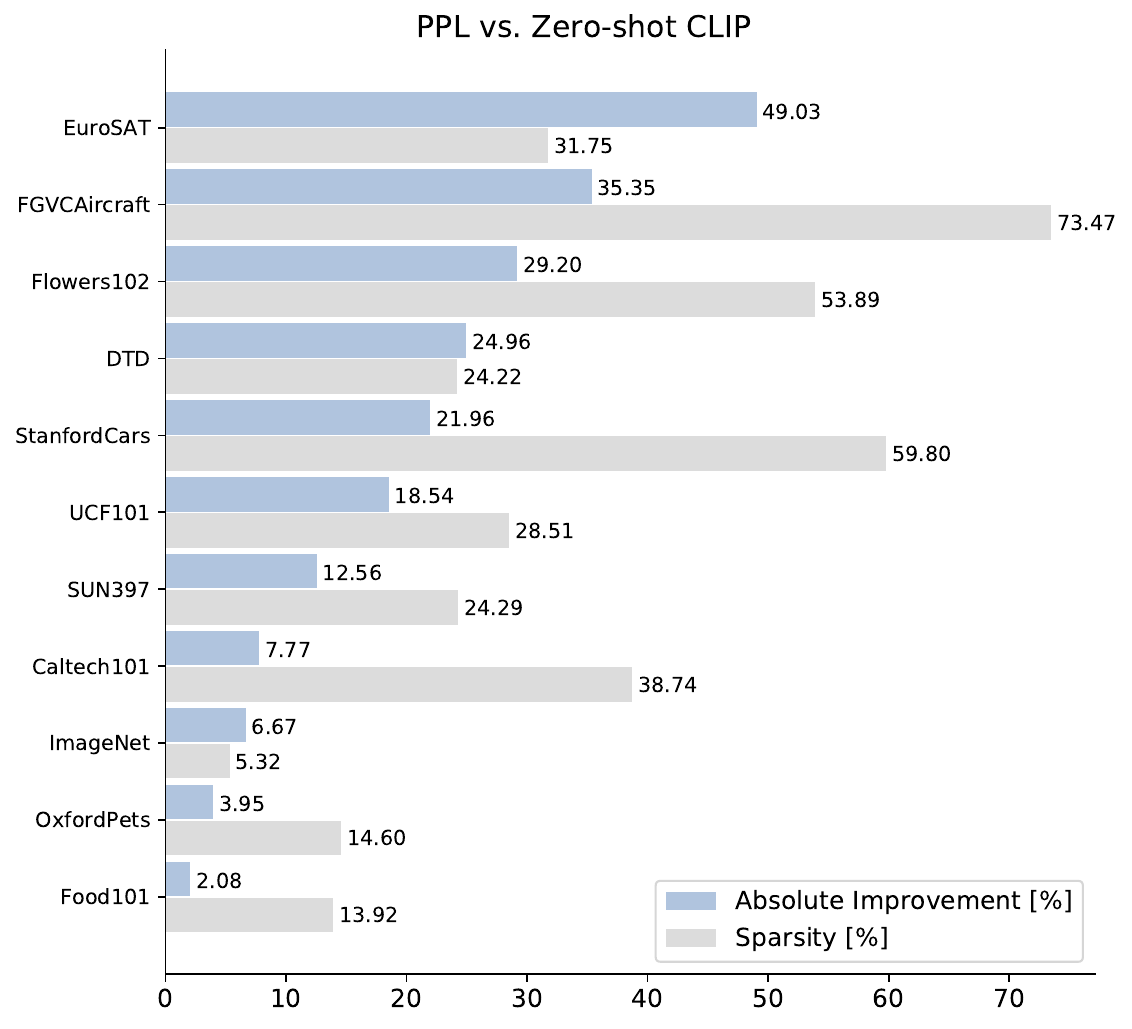}
    \caption{Comparison with Zero-shot CLIP on accuracy and sparsity of image encoder on 16-shot datasets.}
    \label{fig:compare_zs_rn50}
    \vspace{-.1in}
\end{figure}

\section{Combining with state-of-the-art methods}
To prove the PPL is synergistic to existing parameter-efficient methods, we combine it with CoOP~\cite{zhou2022learning} and TIP-Adapter~\cite{zhang2022tip} on 16-shot ImageNet and FGVCAircraft, as shown in~\cref{table:combine_sota}. Particularly, the few-shot training set for PPL, PPL+CoOP, and PPL+TIP-Adapter is the same.
For PPL+CoOP, the learned text prompt is initialized as ``a photo of a [class]''. The length of the text prompt is set to 4. The maximum training epoch is set to be 50 for ImageNet, and 200 for FGCVAircraft, following CoOP~\cite{zhou2022learning}. The results of CoOP reported in~\cref{table:combine_sota} are obtained with the same experimental setting for a fair comparison. The PPL+CoOP boosts the performance of CoOP on ImageNet and FGVCAircraft by 1.79\% and 22.32\%, respectively. The performance degradation of PPL+CoOP compared with PPL may due to overfitting.
For PPL+TIP-Adapter, the $\alpha$ and $\beta$ are set to be 1.0 and 5.5, respectively, following TIP-Adapter~\cite{zhang2022tip}. The adapter is training for 20 epochs. The initial learning rate is set to be 0.001. The hyper-parameter setting for training is the same for TIP-Adapter. The PPL+TIP-Adapter improves TIP-Adapter on 16-shot ImageNet and FGCVAircraft by 1.61\% and 17.38\%, respectively.
This verifies the ability of PPL to endow existing parameter-efficient methods with the ability to better adapt to the downstream task.

\begin{table}[tb]
	\caption{Combining with state-of-the-art methods on 16-shot ImageNet and FGVCAircraft.}
	\centering
	\vspace{-0.20cm}
	\resizebox{2.6in}{!}{
		\begin{tabular}{l|c|c}
		\hline
		\multirow{1}{*}{Methods} & \multirow{1}{*}{ImageNet} & \multirow{1}{*}{FGVCAircraft}\\ 
		\hline 
		
		Zero-shot CLIP & 58.18 & 17.01 \\
		PPL & \textbf{64.85~\textcolor{red}{+ 6.67}} & \textbf{52.36~\textcolor{red}{+ 35.35}}   \\ \hline
		CoOP~\cite{zhou2022learning} & 63.33 & 28.47  \\
		PPL+CoOP & \textbf{65.12~\textcolor{red}{+ 1.79}} & \textbf{50.79 ~\textcolor{red}{+ 22.32}} \\ \hline
		TIP-Adapter~\cite{zhang2022tip} & 64.17* & 35.55 \\
		PPL+TIP-Adapter &\textbf{65.78 ~\textcolor{red}{+ 1.61}} & \textbf{52.93 ~\textcolor{red}{+ 17.38}} \\
		
		\hline
		\end{tabular}
		} 
		\label{table:combine_sota_rn50}
		
	\vspace{-.1in}
	\end{table}

\section{Applying PPL on Text/Image Encoders of CLIP}
% \todo{\cref{table:different_encoder}}

We conduct experiments to analyze the influence of applying PPL on different encoders in CLIP. \cref{table:different_encoder} shows the results on 16-shot FGVCAircraft. The PPL indicates we apply parameter prompts on the image encoder $\boldsymbol{G}_I$. The PPL-T denotes we only train parameter prompts for the text encoder $\boldsymbol{G}_T$ of CLIP, while the PPL-A means we apply parameter prompts on both the image and text encoders. 
However, training parameter prompts for the two encoders simultaneously is hard to converge. We deem this may destroy the affinity between text and image features encoded by CLIP.
Thus, we first train parameter prompts for the image encoder and freeze them for training parameter prompts for the text encoder in PPL-A.
The sparsity of PPL and PPL-T is comparative. But the accuracy improvement is much more significant with PPL. This indicates the unnecessary parameters in the text encoder have less impact on the performance of CLIP compared with the image encoder. Thus, selecting useful parameters in the image encoder for the downstream few-shot classification task makes more sense.
Moreover, the sparsity of parameter prompts for the text encoder is high for PPL-A, but the accuracy decreases. Thus, we only apply parameter prompts on the image encoder of CLIP.

\begin{table}[tb]
	\caption{Influence of applying the mask on different encoders of CLIP on 16-shot FVGCAircraft.}
	
	\centering
	\vspace{-0.20cm}
	\resizebox{\linewidth}{!}{
		\begin{tabular}{c|c|c|c|c}
		\hline
		\multirow{1}{*}{Methods} & \multirow{1}{*}{Zero-shot CLIP} &
		\multirow{1}{*}{PPL} &
		\multirow{1}{*}{PPL-T}&
		\multirow{1}{*}{PPL-A}\\ 
		\hline 
	
		\hline
		Sparsity ($\boldsymbol{G}_T$)  & 0 & 0 &  72.62 & 87.95 \\
		Sparsity ($\boldsymbol{G}_I$)  & 0 & 73.47 &  0 & 73.47 \\
		\hline
		Accuracy & 17.01  & \textbf{52.36}& 39.48 & 50.93 \\
		
		\hline
		\end{tabular}
		}    
		\label{table:different_encoder}
		
	\vspace{-.15in}
	\end{table}

\section{Comparison with Different Prompt-based Methods}
% In Tab. {\color{red}2} of the manuscript paper, we show the main quantitative results based on the ResNet, which mainly compared with the text prompt methods.
% Fig.{\color{red}3} 
In~\cref{fig:main_results} of the manuscript paper, we show the main results based on the ResNet, which mainly compared with the text prompt methods.
To better evaluate the effectiveness of the proposed parameter prompt, we consider comparing the other modality prompt-based methods, \ie, the visual prompt (\ie, VPT) and text/image prompt (\ie, UPT) methods that are designed for the ViT-B/16. 

As shown in~\cref{table:vit}, we show significant improvements in terms of average accuracy compared with the different prompt-based methods (\ie, text prompt--CoOP, image prompt--VPT, and unified prompt--UPT). As we know, existing prompt learning methods mainly introduce the text/image prompts from the input side, which guides the model to learning diverse visual/textual concepts. When the text or image prompts are adopted, the CoOP, VPT, and UPT have more than 11 consistent advantages over the baseline (\ie, Zero-shot CLIP). Except for the input prompts, we design a new type of prompt, termed parameter prompt, which shows outstanding performances over compared methods. This indicates that our parameter prompt learning can lead the pre-trained model to focus on the useful knowledge required by a downstream task.

\begin{table*}[h]
	\caption{Comparison with state-of-the-art methods under 16-shot setting with ViT-B/16 as vision backbone. ``T'', ``V'', ``P'' and ``V \& T'' refer to the text prompt, image prompt, parameter prompt, and unified prompt, respectively.}

	\centering
	% \vspace{-0.20cm}
	\resizebox{\linewidth}{!}{
		\begin{tabular}{l|cccccccccccc}
		\hline
		\makebox[0.05\textwidth][c]{\rotatebox{90}{Method}} &
		\makebox[0.05\textwidth][c]{\rotatebox{90}{ImageNet}} &
		\makebox[0.05\textwidth][c]{\rotatebox{90}{Caltech101}} &
		\makebox[0.05\textwidth][c]{\rotatebox{90}{FGVCAircraft}} &
		\makebox[0.05\textwidth][c]{\rotatebox{90}{StanfordCars}} & 
            \makebox[0.05\textwidth][c]{\rotatebox{90}{Flowers102}} & 
            \makebox[0.05\textwidth][c]{\rotatebox{90}{OxfordPets}} &
		\makebox[0.05\textwidth][c]{\rotatebox{90}{Food101}} &
		\makebox[0.05\textwidth][c]{\rotatebox{90}{DTD}} &
		\makebox[0.05\textwidth][c]{\rotatebox{90}{EuroSAT}} &
		\makebox[0.05\textwidth][c]{\rotatebox{90}{UCF101}} &
		\makebox[0.05\textwidth][c]{\rotatebox{90}{SUN397}} & 
		\makebox[0.05\textwidth][c]{\rotatebox{90}{Average}} \\
 
		\hline 
		ZS. CLIP & 66.73  & 92.94  & 24.72 & 65.32 & 71.34 & 89.21 & 86.06 & 44.39 & 47.60 & 66.75 & 62.50 & 65.23 \\
		CoOP (T) & 71.36 & 95.93 & 38.04 & 77.45 & 95.90 & 92.74 & 86.36 & 68.38 & 78.77 & 82.04 & 73.59 & 78.23 \\
		VPT (V)& 70.57  & 95.83 & 40.96 & 76.13 & 94.96 & 92.91 & 86.18 & 69.79 & \textbf{91.53} & 82.76 & 71.63 & 79.39 \\
		UPT (V\&T)& 72.63 & 95.94 & 46.80 & 84.33 & 97.11 & 92.95 & 85.00 & 70.65 & 90.51 & 84.03 & 75.91 & 81.44 \\
		\hline 
		PPL (P)& \textbf{73.29} & \textbf{96.23} & \textbf{53.42} & \textbf{84.57} & \textbf{97.46} & \textbf{93.49}& \textbf{87.52}& \textbf{74.41} & 89.12 & \textbf{86.55} & \textbf{76.50 } & \textbf{82.96} \\
		Sparsity & 12.97 & 9.53 & 58.05 & 15.99 & 14.10 & 8.20 &6.50 & 8.72  & 1.39 &13.82 & 20.79 & 15.46 \\
		
		\hline
		\end{tabular}
		}    
		\label{table:vit}
% 		\begin{tablenotes}
% 		\scriptsize
% 		\item[*] We use these datasets for few shot image classification task. The number of training data and validation data is set to be a specific multiple of the number of classes in training period. Thus, we only demonstrate the number of testing data.
% 		\end{tablenotes}
		
	% \vspace{-.15in}
	\end{table*}

\noindent
\section{Parameter Prompts on Different Layers.} 
% In \cref{table:layer_sparsity}, we present the sparsity of the parameter prompt on each layer of the image encoder. The models are trained with 16-shots ImageNet and FVGCAircraft. Layer 1-4 denotes the 4 layers in ResNet50 from bottom to up, and SA denotes the last multi-head attention layer. We can observe that the sparsity is relatively higher in the top layers, \eg multi-head attention layer and Layer 4 of ResNet, on both of the datasets. This suggests that knowledge that exists in lower layers is more general than the knowledge in top layers, which is consistent with previous findings~\cite{howard2018universal,mallya2018piggyback,zhao2020masking}.
We consider applying parameter prompts on different layers in the image encoder from top to bottom. The results are demonstrated in \cref{table:layer_ppl}. Layer 1-4 denotes the 4 layers in ResNet50 from bottom to up, and SA denotes the last self-attention layer.
As the number of masked layers increases, the sparsity of parameter prompts become higher. The best accuracy is obtained when parameter prompts are applied on Layer3,4+SA. But it only surpasses applying parameter prompts on all layers by 0.01\%. Thus, we recommend applying parameter prompts on all layers unless the number of training data is too small.
In \cref{fig:grad_cam}, we visualize the image feature maps of Zero-shot CLIP, PPL-SA, and PPL by Grad-CAM~\cite{selvaraju2017grad}. The PPL-SA denotes the parameter prompt is only used on the last self-attention layer. We observe that the parameter prompts lead the model to focus on more regions of the foreground, which demonstrate that the parameter prompts can suppress redundant information.
% and the influence of background is the least when parameter prompts are applied to the whole image encoder.

\begin{table}[tb]
	\caption{Applying the parameter prompt on different layers of image encoder on 16-shot ImageNet.}
	\centering
	\vspace{-0.20cm}
	\resizebox{2.1in}{!}{
		\begin{tabular}{c|c|c}
		\hline
		\multirow{1}{*}{Layers} & \multirow{1}{*}{Accuracy} &
		\multirow{1}{*}{Sparsity} \\ 
		\hline 
		SA &  64.57  & 3.28   \\
		Layer 4+SA &   64.67  &  4.84  \\
		Layer 3,4+SA &  \textbf{64.86} &  4.99  \\
		Layer 2,3,4+SA &  64.79 & 5.05  \\
		All &  64.85 & \textbf{5.32}  \\
		\hline
		\end{tabular}
		} 
		\label{table:layer_ppl}
		
	\vspace{-.15in}
	\end{table}

\section{Different Parameter-Level Prompts}

\begin{table}[h]
	\caption{Different parameter-level prompts on 16-shot ImageNet.}
	\centering
	% \vspace{-0.20cm}
	\resizebox{4.in}{!}{
		\begin{tabular}{c|c|c|c|c|c}
		\hline
		 &\multirow{1}{*}{Zero-shot CLIP}&\multirow{1}{*}{OCPL} &\multirow{1}{*}{ICPL}&\multirow{1}{*}{CPL} &\multirow{1}{*}{PPL}\\ 
		\hline
		Accuracy & 58.18 & 59.35 & 61.57 & 64.67 & 64.85 \\
		Sparsity & 0     & 0.24 & 1.23  & 4.42 & 5.32  \\
		\hline
		\end{tabular}
		} 
		\label{table:mask_channel}
		
\end{table}

Recently, structured network pruning techniques~\cite{liebenwein2019provable,sui2021chip,gao2018dynamic} have been proposed to remove parameters in groups by pruning neurons, filters, channels, or parameters.
Inspired by these network pruning works, we design different prompt learning methods from the dimension aspect, which are classified by Input Channel Prompt Learning (ICPL), Output Channel Prompt Learning (OCPL), Channel Prompt Learning (CPL), and Parameter Prompt Learning (PPL). Concretely, input channel prompt learning is very similar to the channel-wise pruing method that focuses on the pruning of the input channel, while output channel prompt learning is very similar to filter-wise pruning method that focuses on the pruning of output channel. These two prompt learning are with all the details of dependencies reversed. 
Channel prompt learning combines the above prompt learning that masks the input and output channels, simultaneously.
As shown in~\cref{table:mask_channel},  ICPL and OCPL bring relatively low gains in accuracy. It likely neglects some important details in the pre-trained model when we just focus on measuring the importance of channel-wise or filter-wise information.
The best performance is obtained by PPL with highest sparsity on 16-shot ImageNet. The CPL achieves the second best performance, which is 0.18\% lower than PPL. The CPL is similar with PPL.
But the CPL reduces the amount of learnable parameters comparing with PPL when the kernel size of convolutional layer is large than 1. However, we still recommend PPL for better performance.
% the CPL is more practical when the pre-trained model is super-net. But PPL is more useful when combining with ResNet or ViT.
% \todo{wuwei will write this part!!!!!!!!!!!}

\section{Further Analysis of Parameter Prompts}

\noindent\textbf{Sparsity analysis of parameter prompt during training.} We analyze the effectiveness of parameter prompt during training. 
As shown in~\cref{fig:loss} and~\cref{fig:acc}, the accuracy of the model increases with training, while the loss decreases. 
As shown in~\cref{fig:sparsity}, we find that the sparsity of the model increases with the number of layers. This interesting phenomenon indicates that different downstream tasks require more same low-level knowledge in the pre-trained weights. In the high-level layers, the knowledge required by different downstream tasks is semantic inconsistent, and these tasks need different combination of low-level features. Thus, the connections among different neuron (\ie, the parameter prompt) in the high-level layer are more sparse than low-level layer.

\begin{figure*}[h]
    \centering
    \begin{subfigure}[b]{0.33\linewidth}
     \centering
     \includegraphics[width=\linewidth]{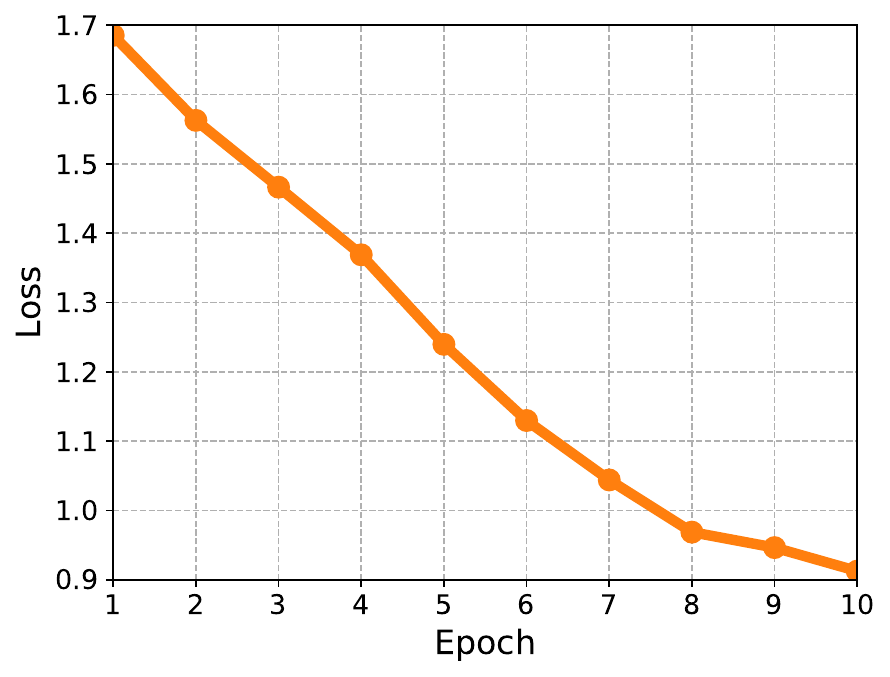}
     \caption{Loss}
     \label{fig:loss}
\end{subfigure}
\begin{subfigure}[b]{0.33\linewidth}
     \centering
     \includegraphics[width=\linewidth]{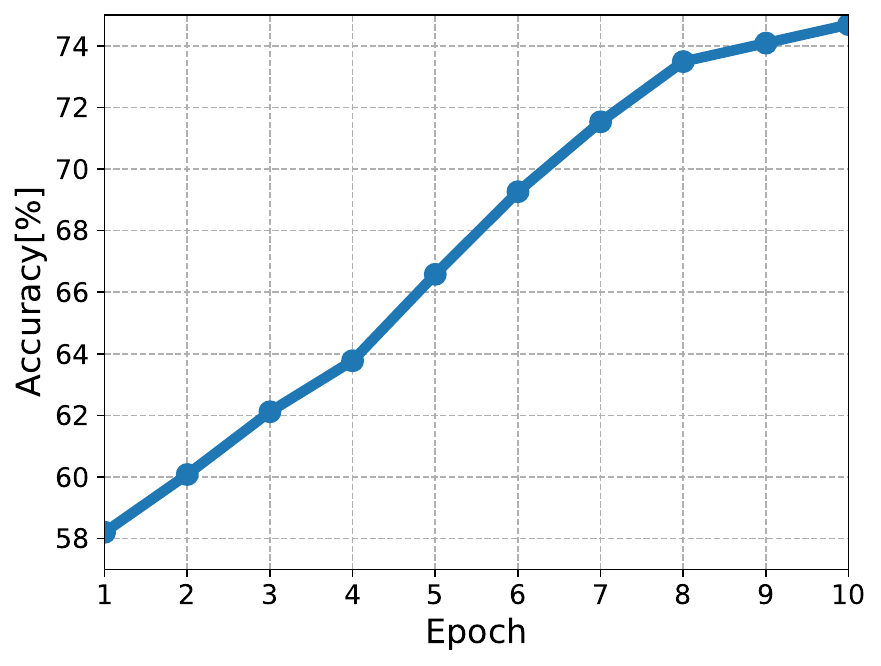}
     \caption{Accuracy on Training Set}
     \label{fig:acc}
\end{subfigure}
\begin{subfigure}[b]{0.33\linewidth}
     \centering
     \includegraphics[width=\linewidth]{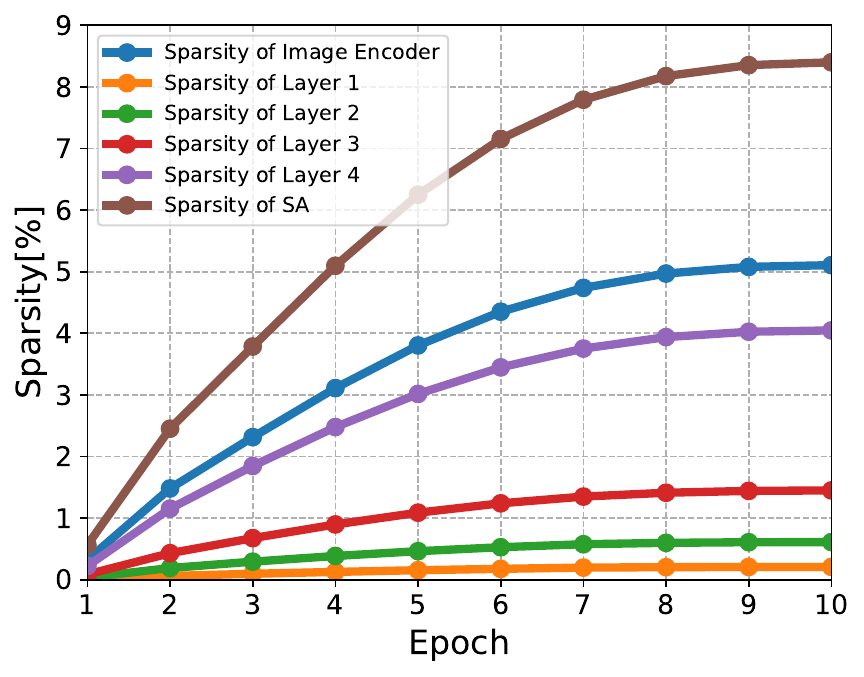}
     \caption{Sparsity}
     \label{fig:sparsity}
\end{subfigure}

\caption{Loss, accuracy on the training set, and sparsity of each layer during the training period, in the 16-shot setting of ImageNet.}
\label{fig:train}
\end{figure*}

\begin{table}[h]
	\caption{Sparsity of parameter prompt on different layers of image encoder on one run of 16-shot ImageNet.}
	\centering
	% \vspace{-0.20cm}
	\resizebox{4.4in}{!}{
		\begin{tabular}{c|c|c|c|c|c|c}
		\hline
		 &\multirow{1}{*}{Layer 1} &\multirow{1}{*}{Layer 2} &\multirow{1}{*}{Layer 3} &\multirow{1}{*}{Layer 4} &\multirow{1}{*}{SA} & \multirow{1}{*}{All}\\ 
		\hline 
		Accuracy &58.44  &58.58 &59.68 &61.69  & 64.22 & 64.92  \\
		Sparsity &0.20 & 0.59 & 1.42 & 4.02 & 8.36 & 5.08  \\
		\hline
		\end{tabular}
		} 
		\label{table:layer_sparsity}
% 	\begin{tablenotes}
% 	    \small
% 	    The quantitative results in manuscript is the average of three runs. Since there are slightly different between 
% 	    The results reported here is from one seed
% 	\end{tablenotes}
		
% 	\vspace{-.1in}
	\end{table} 
\noindent\textbf{Sparsity analysis of parameter prompt on the different layers.} As suggested in~\cref{table:layer_sparsity}, we save the parameter prompts of different layers for evaluation. The quantitative results in the manuscript are the average of three runs. Since there are slight differences between the three runs. To take a close look at the parameter prompts of one image encoder, we only report the results of one run here.
% 	    The results reported here is from one seed
The reported sparsity denotes the sparsity of parameter prompts in each layer. We observe the parameter prompts in low layers, \eg Layer 1/2, are less sparse and have less impact on the transfer capacity of CLIP.

\noindent\textbf{The influence of threshold $\alpha$.} We conduct experiments to analysis the influence of threshold $\alpha$ in~\cref{table:threshold}. The threshold $\alpha$ determines the binarized value in parameter prompts, as shown in~\cref{eq.mask}. %Eq. ({\color{red} 7}). 
We observe the $\alpha$ also influences the sparsity of parameter prompt: when $\alpha$ is larger, the parameter prompt is more sparse. However, the $\alpha$ has less impact on the performance compared with the wight decay $\lambda$. We fix the $\alpha$ as 5e-3 for all experiments.
	
\begin{table}[h]
	\caption{Influence of threshold $\alpha$ on 16-shot ImageNet.}
	\centering
	% \vspace{-0.20cm}
	\resizebox{1.88in}{!}{
		\begin{tabular}{c|c|c}
		\hline
		 \multirow{1}{*}{$\alpha$} &\multirow{1}{*}{Accuracy} &\multirow{1}{*}{Sparsity} \\ 
		\hline 
		6e-3  & 64.74 & 5.83  \\
		5e-3 & 64.85  & 5.32   \\
		4e-3 & 64.78 & 4.39    \\
		\hline
		\end{tabular}
		} 
		\label{table:threshold}
% 	\begin{tablenotes}
% 	    \small
% 	    The quantitative results in manuscript is the average of three runs. Since there are slightly different between 
% 	    The results reported here is from one seed
% 	\end{tablenotes}
		
% 	\vspace{-.1in}
	\end{table}
	
\noindent\textbf{Visualization of parameter prompts.} As shown in~\cref{fig:mask_resnet}, we select a subset of parameter prompts in the vision backbone (\eg, ResNet-50) for visualization. The parameter prompts are learned on 16-shot FGVCAircraft. Due to too many parameters, we only show the visualization of the part parameter prompts. Specifically, in the ResNet-50 backbone, we select the 12 neurons of 0-th, 4-th, 8-th convolution layers in the layer-1, 0-th, 3-th, 7-th, 10-th convolution layers in the layer-2, 0-th, 4-th, 7-th, 11-th, 14-th, 17-th convolution layers in the layer-3, and 0-th, 4-th and 8-th convolution layers in the layer-4.
As analyzed in the same way as the manuscript, the model keeps more connections between different neurons at the low-level layers and more sparsity at the high-level layers.

\begin{figure*}
    \centering
    \includegraphics[width=0.8\linewidth]{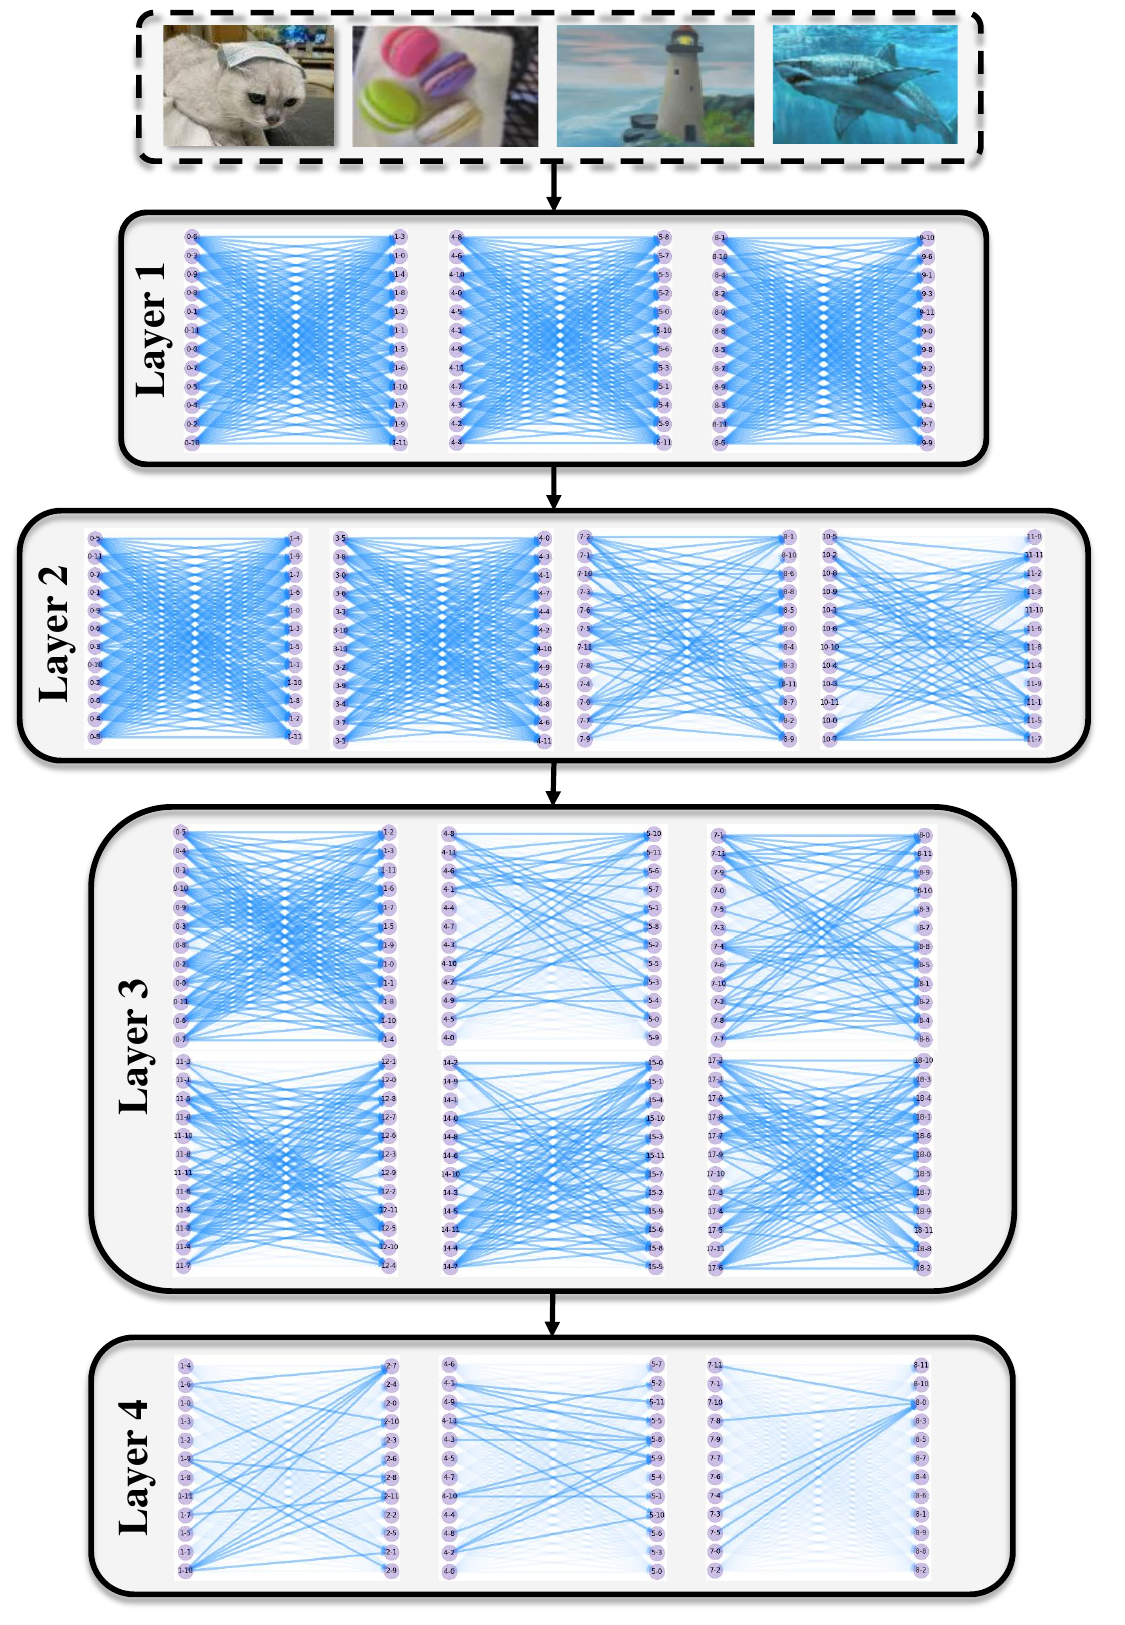}

        \caption{Visualization of a small part of parameter prompts in the vision backbone (\eg, ResNet-50). The parameter prompts are trained on 16-shot FGVCAircraft.}
\label{fig:mask_resnet}
\end{figure*}

\section{Statistic of Datasets}
We conduct experiments on 11 publicly available image classification datasets following CoOP~\cite{zhou2022learning}. The datasets including ImageNet~\cite{deng2009imagenet}, FGVCAircraft~\cite{maji2013fine}, StanfordCars~\cite{Krause_2013_ICCV_Workshops}, Flowers102~\cite{nilsback2008automated}, Caltech101~\cite{fei2004learning}, DTD~\cite{cimpoi2014describing}, EuroSAT~\cite{helber2019eurosat}, Food101~\cite{bossard2014food}, UCF101~\cite{soomro2012ucf101}, OxfordPets~\cite{parkhi2012cats}, and SUN397~\cite{xiao2010sun}. 
We report the detailed statistics of the 11 datasets in \cref{table:dataset}.

\begin{table}[h]
	\caption{The statistics of the 11  image classification datasets}
	\centering
	% \vspace{-0.20cm}
	\resizebox{4.in}{!}{
		\begin{tabular}{c|c|c|c}
		\hline
		\multirow{1}{*}{Dataset} & \multirow{1}{*}{\# of class} &
		\multirow{1}{*}{\# of testing data} &
		\multirow{1}{*}{Task} \\ 
		\hline 
		
		ImageNet~\cite{deng2009imagenet} & 1,000 & 50,000  & Object \\
		Caltech101~\cite{fei2004learning} & 101 & 2,465 & Object \\
		FGVCAircraft~\cite{maji2013fine} & 100 & 3,333  & Fine-grained \\
		StanfordCars~\cite{Krause_2013_ICCV_Workshops} & 196 & 8,041 & Fine-grained \\
		Flowers102~\cite{nilsback2008automated} & 102 & 2,463 & Fine-grained \\
        OxfordPets~\cite{parkhi2012cats} & 37 & 3,669 & Fine-grained \\
        Food101~\cite{bossard2014food} & 101 & 30,300 & Fine-grained \\
		DTD~\cite{cimpoi2014describing} & 47 & 1,692 & Textures \\
		EuroSAT~\cite{helber2019eurosat} & 10 & 8,100 & Satellite Images \\
        UCF101~\cite{soomro2012ucf101} & 101 & 3,783 & Actions \\
		SUN397~\cite{xiao2010sun} & 397 & 19,850 & Scenes \\
		
		\hline
		\end{tabular}
		}    
		\label{table:dataset}
% 		\begin{tablenotes}
% 		\scriptsize
% 		\item[*] We use these datasets for few shot image classification task. The number of training data and validation data is set to be a specific multiple of the number of classes in training period. Thus, we only demonstrate the number of testing data.
% 		\end{tablenotes}
		
	% \vspace{-.15in}
	\end{table}

\section{}{Sparsity Control.}	
For the Adam optimizer, the weight decay $\lambda$ is generally set to be 0. When weight decay is set to be large than 0, it equals adding an L2-regularization term to the loss, which can be formulated as $\lambda\sum_{i,j}m_{i,j}^2$. Thus, we assume that when we set the $\lambda$ to be a large value, the parameters in the learnable matrix $\boldsymbol{M}$ will be fairly small, which results in high sparsity. But if we set the $\lambda$ to be 0, we set no restrictions to the sparsity of the learnable matrix. In this case, the parameter prompts can find a small number of unnecessary parameters within the image encoder. 
Thus, we conduct an ablation study on the weight decay $\lambda$ as shown in \cref{table:wd}. The best performance is obtained when $\lambda=1e-5$.
We observe that when we set $\lambda=1e-4$, the sparsity of parameter prompts increases a lot. The gain diminishes may be caused by leaving out important parameters.
When $\lambda=1e-6$, the sparsity of parameter prompts decreases, and there are still unnecessary parameters that have not been removed in the image encoder.
Thus, the weight decay hyper-parameter $\lambda$ is important for PPL. A suitable weight decay can lead the parameter prompts to find an appropriate sparsity of binary mask, which can leave out unnecessary parameters and keep the important ones.

% \begin{table}[tb]
% 	\caption{Sparsity of parameter prompt on different layers of image encoder on 16-shot ImageNet}
% 	\centering
% 	\vspace{-0.20cm}
% 	\resizebox{\linewidth}{!}{
% 		\begin{tabular}{c|c|c|c|c|c}
% 		\hline
% 		\multirow{1}{*}{Dataset} &\multirow{1}{*}{Layer 1} &\multirow{1}{*}{Layer 2} &\multirow{1}{*}{Layer 3} &\multirow{1}{*}{Layer 4} &\multirow{1}{*}{SA} \\ 
% 		\hline 
% 		ImageNet &0.20 & 0.59 & 1.42 & 4.02 & 8.36 \\
% 		FVGCAircraft & 7.83 & 25.48 & 50.97 & 74.81 & 87.35 \\
% 		\hline
% 		\end{tabular}
% 		} 
% 		\label{table:layer_sparsity}
		
% 	\vspace{-.15in}
% 	\end{table}
	
\begin{table}[tb]
	\caption{Influence of  of optimizer on 16-shot ImageNet.}
	\centering
	\vspace{-0.20cm}
	\resizebox{1.7in}{!}{
		\begin{tabular}{c|c|c}
		\hline
		\multirow{1}{*}{$\lambda$} & \multirow{1}{*}{Accuracy} &
		\multirow{1}{*}{Sparsity} \\ 
		\hline
		1e-6 & 64.78 & 1.02 \\
		1e-5 & 64.85 & 5.32   \\
		1e-4 & 64.45 &  23.64 \\
		\hline
		\end{tabular}
		} 
		\label{table:wd}
		
	\vspace{-.1in}
	\end{table}

\textbf{Parameter Prompts for Different Datasets.} As shown in~\cref{fig:cm}, we present the IoU of parameter prompts between two arbitrary datasets on the 16-shot setting. Since we random sample 16 images per class to train the parameter prompts three times with different seeds, the parameter prompts within one dataset are not always the same. This result demonstrates that for downstream tasks, the knowledge of pre-trained weight is not invariable.
% the average of IoU between parameter prompts trained in two arbitrary runs. 
From \cref{fig:cm}, we also observe that for each dataset the maximum IoU is always itself, which indicates the parameter prompts can find task-specific parameters within CLIP. However, the IoU between some two datasets is relatively high, like ImageNet and Food101. This might result from the similarity in data. The two datasets contain some same categories, \eg, hot dogs and ice cream. Future work may explore the relationship between the parameter prompts and the attribute of datasets.

\begin{figure}[t]
    \centering
    \includegraphics[scale=0.45]{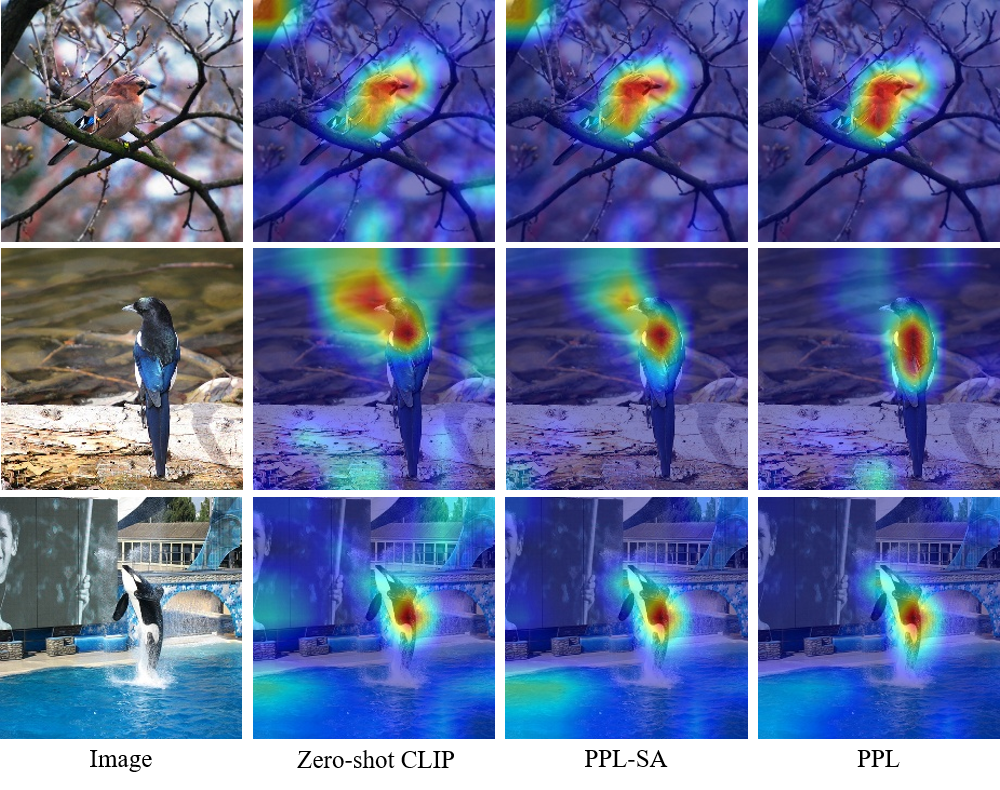}
    \caption{Visualization results of the learned image feature maps on 16-shot ImageNet.}
    \label{fig:grad_cam}
    \vspace{-.15in}
\end{figure}

\begin{figure}[t]
\centering
\includegraphics[scale=0.55]{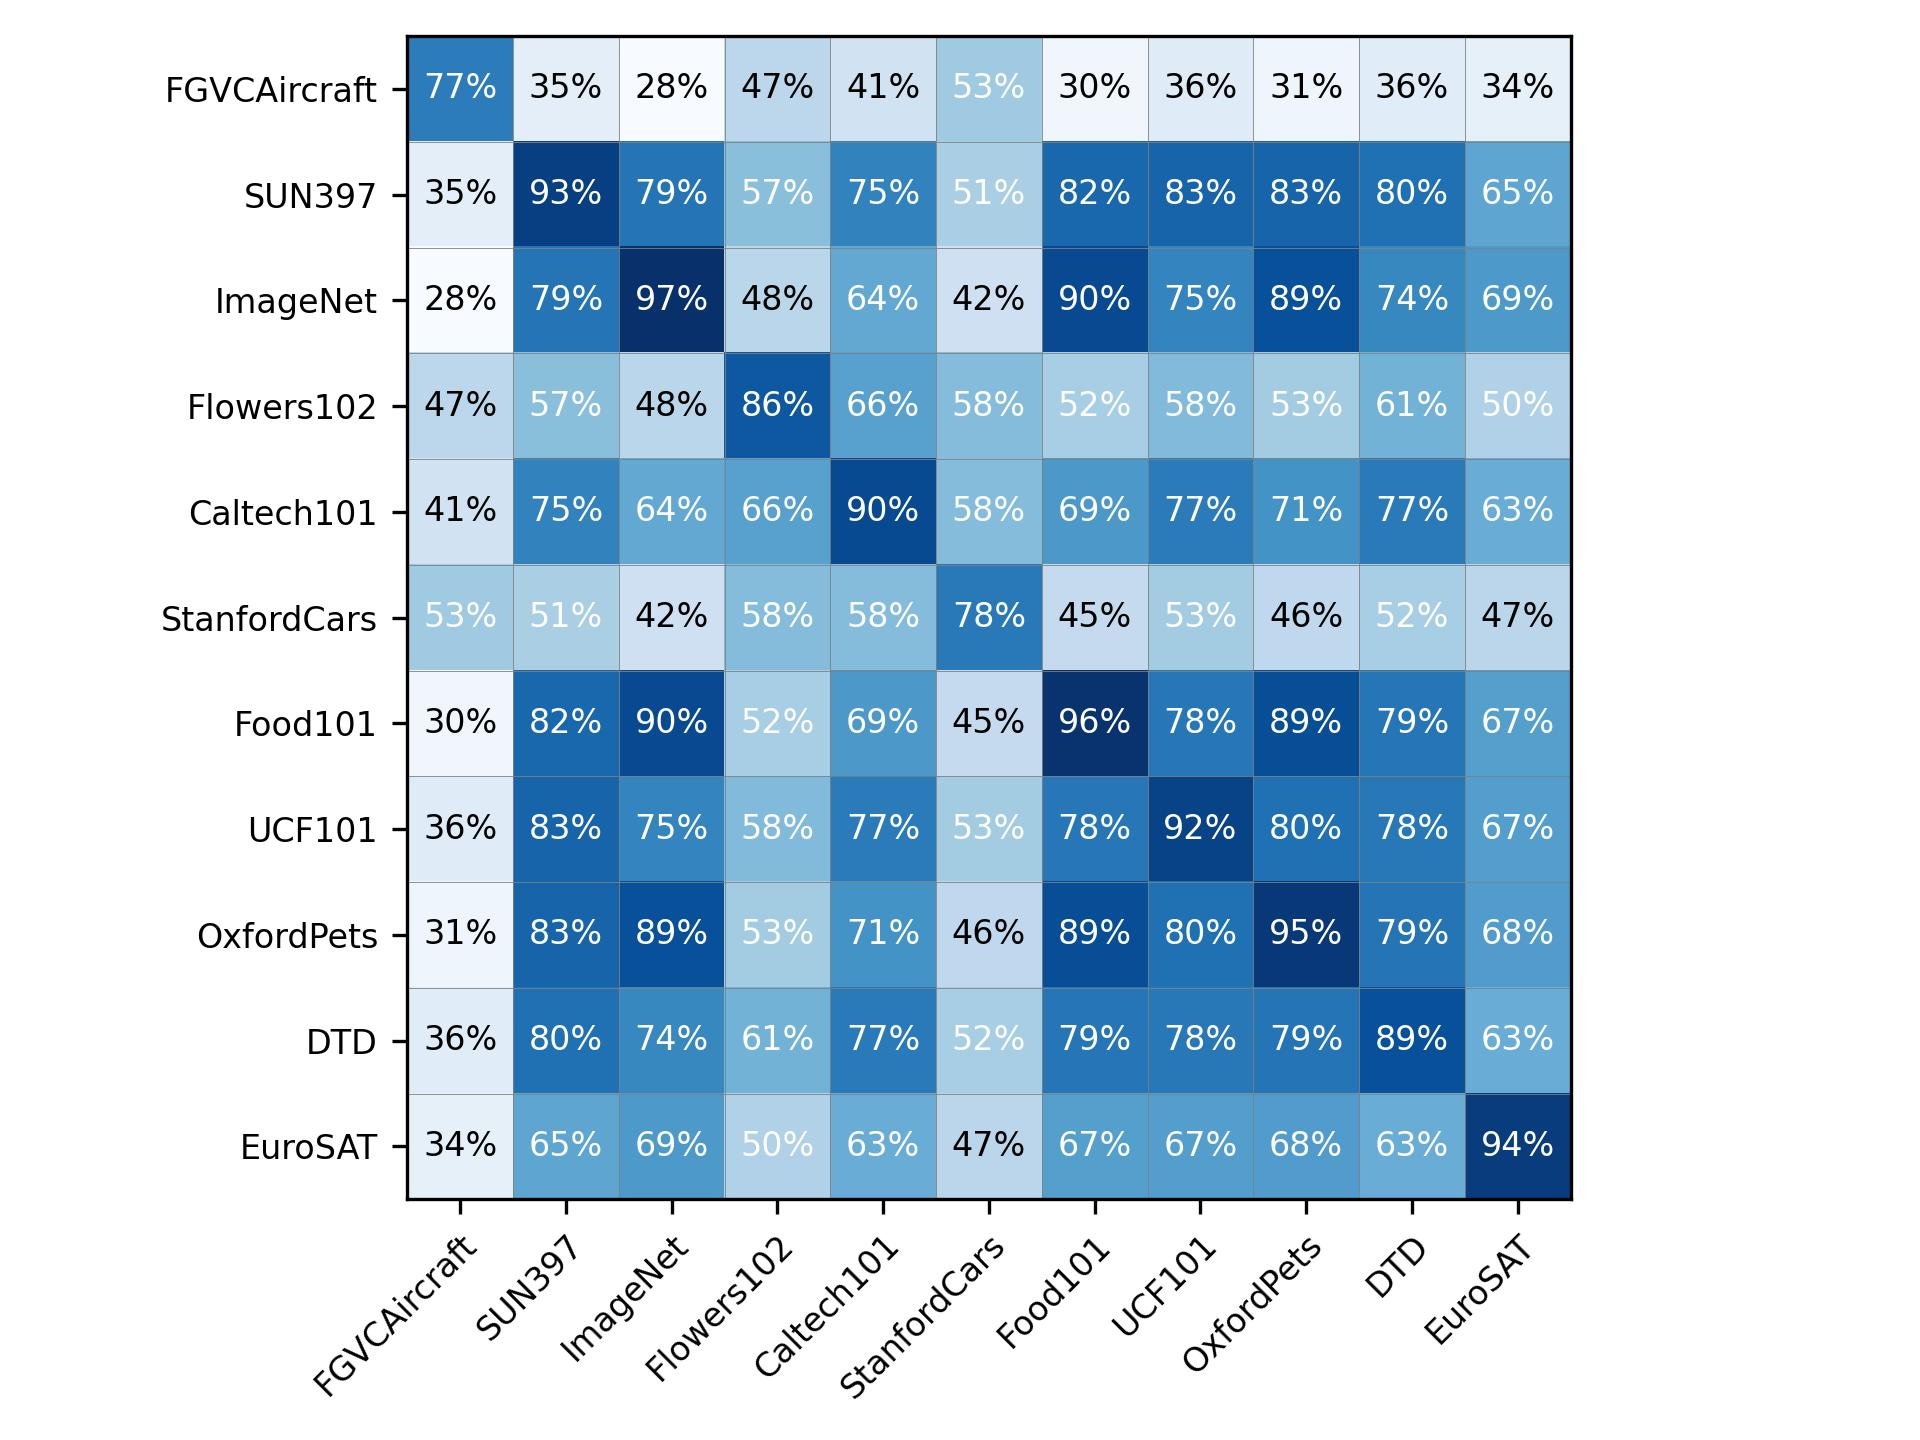}
\caption{IoU between different parameter prompts of 11 datasets.}
\label{fig:cm}
\vspace{-.15in}
\end{figure}

\noindent
\textbf{Different Vision Backbones.} In~\cref{table:vision_backbone}, we report the results of implementing BAT+ and A-BAT+ on different vision backbones of CLIP on 16-shot ImageNet, including ResNet50, ResNet101, ViT-B-16, and ViT-B-32. Concretely, for BAT+, we apply the binary masks on all weight matrices of convolutional layers and fully connected layers.
We can observe that BAT+ achieves the best accuracy on all kinds of vision backbones.
% by leaving out 9.97\% of weight parameters on average.
When utilizing ResNet50, ResNet101, ViT-B-16, and ViT-B-32 as vision backbones, the BAT+ outperforms the second-best method by 0.68\%, 1.13\%, 0.40\%, and 0.88\%, respectively. 
% And PPL exceeds UPT~\cite{zang2022unified} by 0.66\% while using ViT-B-16 as the vision backbone. 
These results demonstrate that the binary tuning is superior to the prompts tuning and adapter tuning.
When using ViT as the visual backbone, A-BAT+ achieves competitive results with BAT+ but introduces fewer parameters. Thus, we still recommend A-BAT+ when ViT is the visual backbone of CLIP.

\begin{table}[tb]
	\caption{Comparison with the state-of-the-art methods with different vision backbones on 16-shot ImageNet.}
	
	\centering
	\vspace{-0.20cm}
	\resizebox{\linewidth}{!}{
		\begin{tabular}{c|c|c|c|c}
		\toprule
		\multirow{1}{*}{Method} & \multirow{1}{*}{ResNet50} &
		\multirow{1}{*}{ResNet101}  &
		\multirow{1}{*}{ViT-B/16}&
		\multirow{1}{*}{ViT-B/32}\\ 
		\hline 
		
		Zero-shot CLIP & 58.18  & 61.62   & 66.73 &  62.05 \\
		VPT~\cite{jia2022visual} & - & - & 70.57 &- \\
		CoOP~\cite{zhou2022learning} & 62.90 & 66.60 & 71.92& 66.85  \\
		CLIP-Adapter~\cite{gao2021clip} & 63.59  & 65.39  & 71.13 & 66.19  \\
		TIP-Adapter~\cite{zhang2022tip} & 64.17 & 66.42  & 73.08 &  67.12 \\
		UPT~\cite{zang2022unified} & - & - & 72.63 &- \\
            % ProDA~\cite{lu2022prompt} &  65.30 & - & - & - \\
            PLOT+CoOP~\cite{chen2022prompt} & 63.01 & - & - & -\\
            % PLOT+TIP-Adapter~\cite{chen2022prompt} & 66.17 & - & - & -\\
		\hline
            A-BAT+ & - & - & 73.07 & 67.84 \\
		BAT+ & \textbf{64.85~\textcolor{red}{+0.68}} & \textbf{67.73~\textcolor{red}{+1.13}}  & \textbf{73.48~\textcolor{red}{+0.40}} & \textbf{68.00~\textcolor{red}{+0.88}}  \\
		% Sparisty & 5.32 & 9.80  & 12.97   & 11.80  \\
		\bottomrule
		\end{tabular}
		}  
		% \begin{tablenotes}
  %   		\scriptsize
  %   		\item[*] For TIP-Adapter, the results reported by Zhang \etal~\cite{zhang2022tip} on ImageNet are based on using prompt ensembling as text input. For a fair comparison, we conduct experiments with a single text prompt for TIP-Adapter and report the results here.
		% \end{tablenotes}
		\label{table:vision_backbone}
		
	\vspace{-.1in}
\end{table}

\begin{figure}[t]
    \centering
    \includegraphics[scale=0.4]{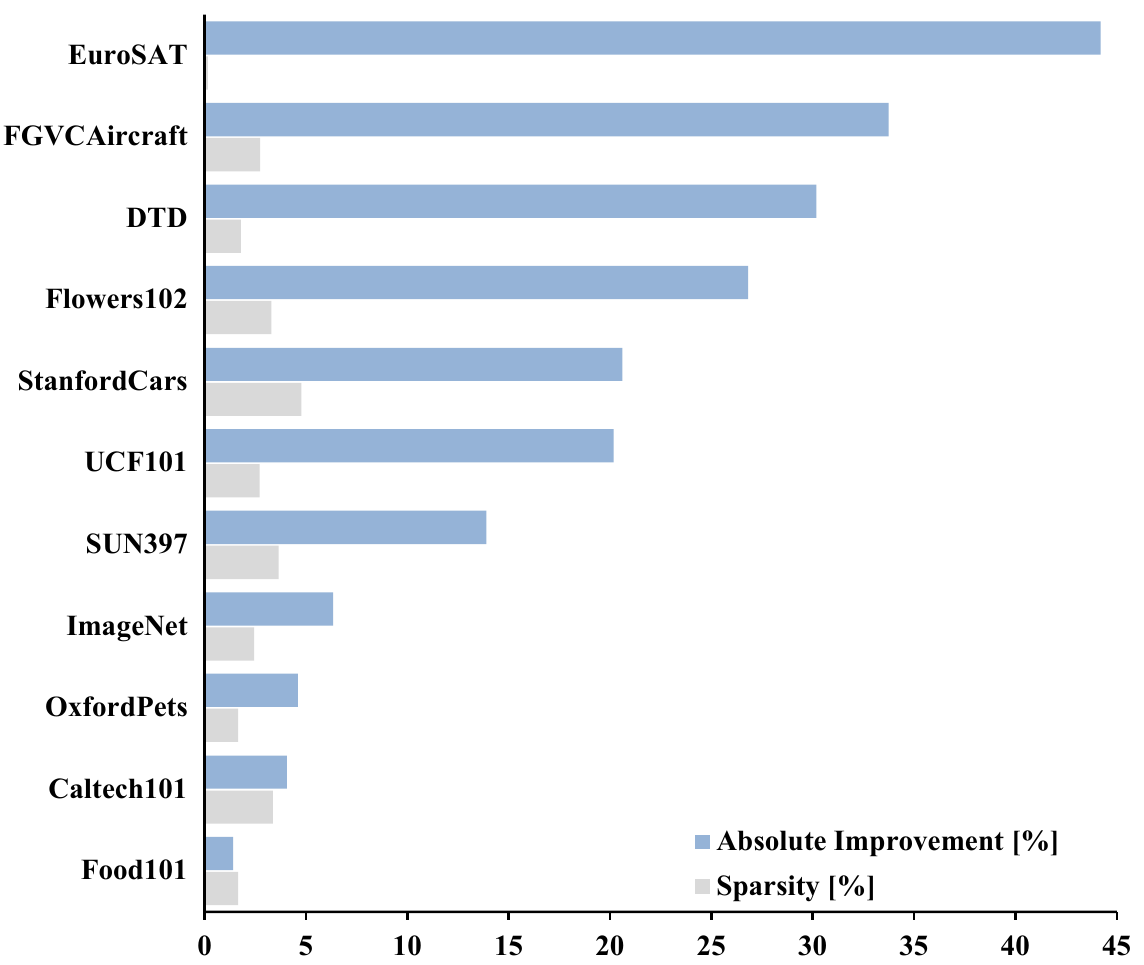}
    \caption{Comparison with Zero-shot CLIP in terms of accuracy and sparsity on 16-shot datasets. The sparsity means the percentage of the number of discarded parameters (mask=0).
     % out of the total number of parameters of the image encoder
    }
    \label{fig:compare_zs_vit}
    \vspace{-.1in}
\end{figure}

\paragraph{Comparison with Zero-shot CLIP}
In \cref{fig:compare_zs_vit}, we demonstrate the absolute improvement of R-AMT compared with Zero-shot CLIP and the sparsity of binary masks on the 16-shot setting. The R-AMT boosts the performance of Zero-shot CLIP on all datasets. Significant improvements are achieved on the EuroSAT and FGVCAircraft datasets, which reach 44.20\% and 33.75\%, respectively. 
The most sparse binary mask is obtained on StanfordCars. After setting 4.77\% parameters to 0, the R-AMT improves Zero-shot CLIP 20.61\% on accuracy.
It proves that the pre-trained weights contain some unnecessary information for the downstream task, which may harm the transfer ability of the pre-trained model.
